# Supplementary material for: Investigating the Effectiveness of HyperTuning via Gisting
Source: arXiv:2402.16817 source file (2024-02-26)
Supplement: Supplementary file 1 [file p3train.tex]

\begin{figure}
\begin{minipage}[t]{\linewidth}\raggedright
\tiny{adversarial\_qa\_dbert\_answer\_the\_following\_q, adversarial\_qa\_dbert\_based\_on, adversarial\_qa\_dbert\_generate\_question, adversarial\_qa\_dbert\_question\_context\_answer, adversarial\_qa\_dbert\_tell\_what\_it\_is, adversarial\_qa\_dbidaf\_answer\_the\_following\_q, adversarial\_qa\_dbidaf\_based\_on, adversarial\_qa\_dbidaf\_generate\_question, adversarial\_qa\_dbidaf\_question\_context\_answer, adversarial\_qa\_dbidaf\_tell\_what\_it\_is, adversarial\_qa\_droberta\_answer\_the\_following\_q, adversarial\_qa\_droberta\_based\_on, adversarial\_qa\_droberta\_generate\_question, adversarial\_qa\_droberta\_question\_context\_answer, adversarial\_qa\_droberta\_tell\_what\_it\_is, ag\_news\_classify, ag\_news\_classify\_question\_first, ag\_news\_classify\_with\_choices, ag\_news\_classify\_with\_choices\_question\_first, ag\_news\_recommend, ag\_news\_which\_section, ag\_news\_which\_section\_choices, amazon\_polarity\_Is\_this\_product\_review\_positive, amazon\_polarity\_Is\_this\_review, amazon\_polarity\_Is\_this\_review\_negative, amazon\_polarity\_User\_recommend\_this\_product, amazon\_polarity\_convey\_negative\_or\_positive\_sentiment, amazon\_polarity\_flattering\_or\_not, amazon\_polarity\_negative\_or\_positive\_tone, amazon\_polarity\_user\_satisfied, amazon\_polarity\_would\_you\_buy, app\_reviews\_categorize\_rating\_using\_review, app\_reviews\_convert\_to\_rating, app\_reviews\_convert\_to\_star\_rating, app\_reviews\_generate\_review, cnn\_dailymail\_3.0.0\_generate\_story, cnn\_dailymail\_3.0.0\_spice\_up\_story, common\_gen\_Example\_prompt, common\_gen\_Given\_concepts\_type\_1, common\_gen\_Given\_concepts\_type\_2, common\_gen\_Put\_together, common\_gen\_choice\_in\_concept\_centric\_sentence\_generation, common\_gen\_random\_task\_template\_prompt, common\_gen\_sentence\_to\_concepts, common\_gen\_topic\_to\_sentence, common\_gen\_topics\_from\_the\_sentence, cos\_e\_v1.11\_aligned\_with\_common\_sense, cos\_e\_v1.11\_description\_question\_option\_id, cos\_e\_v1.11\_description\_question\_option\_text, cos\_e\_v1.11\_explain\_why\_human, cos\_e\_v1.11\_generate\_explanation\_given\_text, cos\_e\_v1.11\_i\_think, cos\_e\_v1.11\_question\_description\_option\_id, cos\_e\_v1.11\_question\_description\_option\_text, cos\_e\_v1.11\_question\_option\_description\_id, cos\_e\_v1.11\_question\_option\_description\_text, cos\_e\_v1.11\_rationale, cosmos\_qa\_context\_answer\_to\_question, cosmos\_qa\_context\_description\_question\_answer\_id, cosmos\_qa\_context\_description\_question\_answer\_text, cosmos\_qa\_context\_description\_question\_text, cosmos\_qa\_context\_question\_description\_answer\_id, cosmos\_qa\_context\_question\_description\_answer\_text, cosmos\_qa\_context\_question\_description\_text, cosmos\_qa\_description\_context\_question\_answer\_id, cosmos\_qa\_description\_context\_question\_answer\_text, cosmos\_qa\_description\_context\_question\_text, cosmos\_qa\_no\_prompt\_id, cosmos\_qa\_no\_prompt\_text, cosmos\_qa\_only\_question\_answer, dbpedia\_14\_given\_a\_choice\_of\_categories\_, dbpedia\_14\_given\_a\_list\_of\_category\_what\_does\_the\_title\_belong\_to, dbpedia\_14\_given\_list\_what\_category\_does\_the\_paragraph\_belong\_to, dbpedia\_14\_pick\_one\_category\_for\_the\_following\_text, dream\_answer\_to\_dialogue, dream\_baseline, dream\_generate\_first\_utterance, dream\_generate\_last\_utterance, dream\_read\_the\_following\_conversation\_and\_answer\_the\_question, duorc\_ParaphraseRC\_build\_story\_around\_qa, duorc\_SelfRC\_build\_story\_around\_qa, gigaword\_TLDR, gigaword\_first\_sentence\_title, gigaword\_generate\_summary\_for\_this, gigaword\_in\_a\_nutshell, gigaword\_make\_a\_title, gigaword\_reverse\_writing, gigaword\_write\_a\_title\_for\_this\_sentence, gigaword\_write\_an\_article, gigaword\_write\_its\_sentence, glue\_mrpc\_equivalent, glue\_mrpc\_generate\_paraphrase, glue\_mrpc\_generate\_sentence, glue\_mrpc\_paraphrase, glue\_mrpc\_replace, glue\_mrpc\_same\_thing, glue\_mrpc\_want\_to\_know, glue\_qqp\_answer, glue\_qqp\_duplicate, glue\_qqp\_duplicate\_or\_not, glue\_qqp\_meaning, glue\_qqp\_quora, glue\_qqp\_same\_thing, imdb\_Movie\_Expressed\_Sentiment, imdb\_Movie\_Expressed\_Sentiment\_2, imdb\_Negation\_template\_for\_positive\_and\_negative, imdb\_Reviewer\_Enjoyment, imdb\_Reviewer\_Enjoyment\_Yes\_No, imdb\_Reviewer\_Expressed\_Sentiment, imdb\_Reviewer\_Opinion\_bad\_good\_choices, imdb\_Reviewer\_Sentiment\_Feeling, imdb\_Sentiment\_with\_choices\_, imdb\_Text\_Expressed\_Sentiment, imdb\_Writer\_Expressed\_Sentiment, kilt\_tasks\_hotpotqa\_combining\_facts, kilt\_tasks\_hotpotqa\_complex\_question, kilt\_tasks\_hotpotqa\_final\_exam, kilt\_tasks\_hotpotqa\_formulate, kilt\_tasks\_hotpotqa\_straighforward\_qa, paws\_labeled\_final\_Concatenation, paws\_labeled\_final\_Concatenation\_no\_label, paws\_labeled\_final\_Meaning, paws\_labeled\_final\_Meaning\_no\_label, paws\_labeled\_final\_PAWS\_ANLI\_GPT3, paws\_labeled\_final\_PAWS\_ANLI\_GPT3\_no\_label, paws\_labeled\_final\_Rewrite, paws\_labeled\_final\_Rewrite\_no\_label, paws\_labeled\_final\_context\_question, paws\_labeled\_final\_context\_question\_no\_label, paws\_labeled\_final\_paraphrase\_task, paws\_labeled\_final\_task\_description\_no\_label, qasc\_is\_correct\_1, qasc\_is\_correct\_2, qasc\_qa\_with\_combined\_facts\_1, qasc\_qa\_with\_separated\_facts\_1, qasc\_qa\_with\_separated\_facts\_2, qasc\_qa\_with\_separated\_facts\_3, qasc\_qa\_with\_separated\_facts\_4, qasc\_qa\_with\_separated\_facts\_5, quarel\_choose\_between, quarel\_do\_not\_use, quarel\_heres\_a\_story, quarel\_logic\_test, quarel\_testing\_students, quartz\_answer\_question\_based\_on, quartz\_answer\_question\_below, quartz\_given\_the\_fact\_answer\_the\_q, quartz\_having\_read\_above\_passage, quartz\_paragraph\_question\_plain\_concat, quartz\_read\_passage\_below\_choose, quartz\_use\_info\_from\_paragraph\_question, quartz\_use\_info\_from\_question\_paragraph, ropes\_background\_new\_situation\_answer, ropes\_background\_situation\_middle, ropes\_given\_background\_situation, ropes\_new\_situation\_background\_answer, ropes\_plain\_background\_situation, ropes\_plain\_bottom\_hint, ropes\_plain\_no\_background, ropes\_prompt\_beginning, ropes\_prompt\_bottom\_hint\_beginning, ropes\_prompt\_bottom\_no\_hint, ropes\_prompt\_mix, ropes\_read\_background\_situation, rotten\_tomatoes\_Movie\_Expressed\_Sentiment, rotten\_tomatoes\_Movie\_Expressed\_Sentiment\_2, rotten\_tomatoes\_Reviewer\_Enjoyment, rotten\_tomatoes\_Reviewer\_Enjoyment\_Yes\_No, rotten\_tomatoes\_Reviewer\_Expressed\_Sentiment, rotten\_tomatoes\_Reviewer\_Opinion\_bad\_good\_choices, rotten\_tomatoes\_Reviewer\_Sentiment\_Feeling, rotten\_tomatoes\_Sentiment\_with\_choices\_, rotten\_tomatoes\_Text\_Expressed\_Sentiment, rotten\_tomatoes\_Writer\_Expressed\_Sentiment, samsum\_Generate\_a\_summary\_for\_this\_dialogue, samsum\_Given\_the\_above\_dialogue\_write\_a\_summary, samsum\_Sum\_up\_the\_following\_dialogue, samsum\_Summarize\_, samsum\_Summarize\_this\_dialogue\_, samsum\_To\_sum\_up\_this\_dialog, samsum\_Write\_a\_dialogue\_that\_match\_this\_summary, sciq\_Direct\_Question, sciq\_Direct\_Question\_Closed\_Book\_, sciq\_Multiple\_Choice, sciq\_Multiple\_Choice\_Closed\_Book\_, sciq\_Multiple\_Choice\_Question\_First, social\_i\_qa\_Check\_if\_a\_random\_answer\_is\_valid\_or\_not, social\_i\_qa\_Generate\_answer, social\_i\_qa\_Generate\_the\_question\_from\_the\_answer, social\_i\_qa\_I\_was\_wondering, social\_i\_qa\_Show\_choices\_and\_generate\_answer, social\_i\_qa\_Show\_choices\_and\_generate\_index, trec\_fine\_grained\_ABBR, trec\_fine\_grained\_ABBR\_context\_first, trec\_fine\_grained\_DESC, trec\_fine\_grained\_DESC\_context\_first, trec\_fine\_grained\_ENTY, trec\_fine\_grained\_HUM, trec\_fine\_grained\_HUM\_context\_first, trec\_fine\_grained\_LOC, trec\_fine\_grained\_LOC\_context\_first, trec\_fine\_grained\_NUM, trec\_fine\_grained\_NUM\_context\_first, trec\_fine\_grained\_open, trec\_fine\_grained\_open\_context\_first, trec\_pick\_the\_best\_descriptor, trec\_trec1, trec\_trec2, trec\_what\_category\_best\_describe, trec\_which\_category\_best\_describes, wiki\_bio\_comprehension, wiki\_bio\_guess\_person, wiki\_bio\_key\_content, wiki\_bio\_what\_content, wiki\_bio\_who, wiki\_qa\_Decide\_good\_answer, wiki\_qa\_Direct\_Answer\_to\_Question, wiki\_qa\_Generate\_Question\_from\_Topic, wiki\_qa\_Is\_This\_True\_, wiki\_qa\_Jeopardy\_style, wiki\_qa\_Topic\_Prediction\_Answer\_Only, wiki\_qa\_Topic\_Prediction\_Question\_Only, wiki\_qa\_Topic\_Prediction\_Question\_and\_Answer\_Pair, wiki\_qa\_automatic\_system, wiki\_qa\_exercise, wiki\_qa\_found\_on\_google, wiqa\_does\_the\_supposed\_perturbation\_have\_an\_effect, wiqa\_effect\_with\_label\_answer, wiqa\_effect\_with\_string\_answer, wiqa\_what\_is\_the\_final\_step\_of\_the\_following\_process, wiqa\_what\_is\_the\_missing\_first\_step, wiqa\_what\_might\_be\_the\_first\_step\_of\_the\_process, wiqa\_what\_might\_be\_the\_last\_step\_of\_the\_process, wiqa\_which\_of\_the\_following\_is\_the\_supposed\_perturbation, yelp\_review\_full\_based\_on\_that, yelp\_review\_full\_format\_rating, yelp\_review\_full\_format\_score, yelp\_review\_full\_format\_star, yelp\_review\_full\_on\_a\_scale, yelp\_review\_full\_so\_i\_would, yelp\_review\_full\_this\_place
}
\end{minipage}
\caption{List of P3 dataset-prompts used for training. We chose a subset of T0-train with average input lengths shorter than 320 tokens.}
\label{fig:appp3train}
\end{figure}
