# Supplementary material for: Investigating the Effectiveness of HyperTuning via Gisting
Source: arXiv:2402.16817 source file (2024-02-26)
Supplement: Supplementary file 2 [file pseudocode.tex]

\begin{figure}
\begin{lstlisting}
# B = batch_size
# T = input_length
# P = number of prompt tokens
# H = hidden_dim
# L = num layers in encoder/decoder

# Shape: [B, T]
fewshot_input_ids = ...

# Shape: [B, T, H]
hyper_enc_out = hypermodel.encoder(fewshot_input_ids)

# Shape: [B, 2P, H]
# Decoder implicitly uses a fixed set of input embeddings of size 2P
hyper_dec_out = hypermodel.decoder(hyper_enc_out)

# Shape: [B, P, LH]
downstream_enc_k_prefix = hypermodel.enc_k_head(hyper_dec_out[:, :P, :])
downstream_enc_v_prefix = hypermodel.enc_v_head(hyper_dec_out[:, :P, :])
downstream_dec_k_prefix = hypermodel.dec_k_head(hyper_dec_out[:, P:, :])
downstream_dec_v_prefix = hypermodel.dec_v_head(hyper_dec_out[:, P:, :])

# Shape: [B, P, L H]
downstream_enc_k_prefix = downstream_enc_k_prefix.reshape(B, P, L, H)
downstream_enc_v_prefix = downstream_enc_v_prefix.reshape(B, P, L, H)
downstream_dec_k_prefix = downstream_dec_k_prefix.reshape(B, P, L, H)
downstream_dec_v_prefix = downstream_dec_v_prefix.reshape(B, P, L, H)
# These correspond to the per-layer learned prefixes for K and V


# where each of the heads is defined (e.g.):
hypermode.enc_k_head = nn.Sequential([
    nn.LayerNorm(),
    nn.Linear(H),
    nn.TanH(),
    nn.Linear(L*H),
])
\end{lstlisting}
\caption{Pseudo-code for HyperT5-Prefix}
\label{app:pseudoprefix}
\end{figure}

\begin{figure}
\begin{lstlisting}
# B = batch_size
# T = input_length
# R = LoRA rank
# H = hidden_dim
# L = num layers in encoder/decoder

# Shape: [B, T]
fewshot_input_ids = ...

# Shape: [B, T, H]
hyper_enc_out = hypermodel.encoder(fewshot_input_ids)

# Shape: [B, 3L, H]
# Decoder implicitly uses a fixed set of input embeddings of size 3L
hyper_dec_out = hypermodel.decoder(hyper_enc_out)

# Shape: [B, L, H]
enc_repr = hyper_dec_out[:, :L, :]
dec_repr = hyper_dec_out[:, L:2*L, :]
cross_repr = hyper_dec_out[:, 2*L:, :]

# Repeat for dec_repr, cross_repr for decoder self- and cross-attention
# Shape: [B, L, 2RH]
enc_q_repr = hypermodel.enc_q_head(enc_repr)
enc_v_repr = hypermodel.enc_v_head(enc_repr)

# Shape: [B, L, 2RH]
enc_q_repr = enc_q_repr.reshape(B, L, 2, R, H)
enc_v_repr = enc_v_repr.reshape(B, L, 2, R, H)

# raw_enc_q_gate and raw_enc_v_gate are learned parameters of size [L]
# Shape: [1, L, 1, 1, 1]
enc_q_gate = torch.tanh(raw_enc_q_gate)[None, :, None, None, None]
enc_v_gate = torch.tanh(raw_enc_v_gate)[None, :, None, None, None]

# Shape: List of [B, R, H]
enc_lora_q_up_list = [enc_q_repr[:, l, 0, :, :] for l in range(L)]
enc_lora_q_down_list = [enc_q_repr[:, l, 1, :, :] for l in range(L)]
enc_lora_v_up_list = [enc_v_repr[:, l, 0, :, :] for l in range(L)]
enc_lora_v_down_list = [enc_v_repr[:, l, 1, :, :] for l in range(L)]
# These correspond to up- and down-map deltas in LoRA in Q and V 
# attention linear maps


# where each of the heads is defined (e.g.):
hypermode.enc_q_head = nn.Sequential([
    nn.LayerNorm(),
    nn.Linear(H),
    nn.TanH(),
    nn.Linear(2*R*H),
])
\end{lstlisting}
\caption{Pseudo-code for HyperT5-LoRA}
\label{app:pseudolora}
\end{figure}
